# Supplementary material for: Gelling by Heating
Source: arXiv:1303.2582 ancillary file (2013-03-11)
Supplement: Supplementary file 1 [file supp_inf.pdf]

# Gelling by Heating: Supplementary Information

Sándalo Roldán-Vargas[1], Frank Smallenburg[1], Walter Kob[2], Francesco Sciortino[1]
[1]*Department of Physics, Sapienza, Università di Roma, Piazzale Aldo Moro 2, I-00185, Roma, Italy,*
[2]*Laboratoire Charles Coulomb, UMR 5221, CNRS and Université Montpellier 2, Montpellier, France*

## MODEL

The particles investigated in the paper are modeled via the well-known Kern-Frenkel model [1]. In this model, particles interact by means of a combination of a hard-sphere potential $u_{\rm HS}$ and an attractive directional interaction $u_{\rm patch}$. The hard-core repulsion between two particles $i$ and $j$ is given by:

$$\beta u_{\rm HS}(r_{ij}) = \begin{cases} \infty & \text{if } r < \sigma_{ij} \\ 0 & \text{otherwise} \end{cases}, \tag{1}$$

Here, $\beta = 1/k_B T$, with $k_B$ Boltzmann's constant and $T$ the temperature, $r_{ij}$ is the center-to-center distance between the particles, and $\sigma_{ij} = (\sigma_i + \sigma_j)/2$ denotes the contact distance between the particles, with $\sigma_i(\sigma_j)$ the diameter of particle $i(j)$. The site-specific attraction between the particles is determined by the circular patches on the surface of each particle, which interact such that two particles form a bond with interaction energy $\epsilon_{ij}$ when i) their centers of mass are within a maximum interaction range $\sigma_{ij} + \delta_{ij}$, and ii) the center-to-center vector between the particles passes through a patch on the surface of both particles (see Fig. 1 of main text). The size of the patches is determined by an opening angle $\theta_{ij}$. The potential energy of two particles $i$ and $j$ is thus given by

$$u_{\rm patch}(\mathbf{r}_{ij}, \{\mathbf{p}_i\}, \{\mathbf{p}_j\}) = u_{\rm SW}(r_{ij})\Phi(\mathbf{r}_{ij}, \{\mathbf{p}_i\})\Phi(\mathbf{r}_{ji}, \{\mathbf{p}_j\}), \tag{2}$$

where $u_{\rm SW}$ is a square-well attraction, given by:

$$u_{\rm SW}(r_{ij}) = \begin{cases} -\epsilon & \text{if } r_{ij} < \sigma_{ij} + \delta_{ij} \\ 0 & \text{otherwise} \end{cases} \tag{3}$$

The function $\Phi(\mathbf{r}_{ij}, \{\mathbf{p}_i\})$ is defined as

$$\Phi(\mathbf{r}_{ij}, \{\mathbf{p}_i\}) = \begin{cases} 1 & \text{if } \hat{\mathbf{r}}_{ij} \cdot \mathbf{p} > \cos(\theta_{ij}) \text{ for any } \mathbf{p} \text{ in } \{\mathbf{p}_i\} \\ 0 & \text{otherwise} \end{cases} \tag{4}$$

where $\mathbf{r}_{ij} = \mathbf{r}_j - \mathbf{r}_i$, $\{\mathbf{p}_i\}$ is a set of normalized vectors pointing from the center of particle $i$ towards the center of each of its patches, and $\hat{\mathbf{r}}$ is a unit vector in the direction of $\mathbf{r}$.

In the model used in the Letter, all particles are either species $A$ or species $B$. The $A$-particles (with hard sphere diameter $\sigma_A$) have four patches each, arranged in a tetrahedral geometry. The $B$-particles are smaller, with $\sigma_B = 0.35\sigma_A$, and have only a single patch. The parameters for the interaction between two $A$-particles are given by $\cos\theta_{AA} = 0.92$, and $\delta_{AA} = 0.15\sigma_A$. For the $AB$-interactions, $\cos\theta_{AB} = 0.99$, and $\delta_{AB} = 0.2\sigma_A$. There are no attractive interactions between the $B$-particles. The ratio between the two interaction strengths is fixed at $\epsilon_{AA} = 0.95\epsilon_{AB}$.

## EVENT-DRIVEN MOLECULAR DYNAMICS

To study the relaxation dynamics of our model we use event-driven Molecular Dynamics (EDMD) simulations [2, 3]. The implementation of the EDMD simulation relies on the numerical prediction of bond formation and bond breaking events, and follows the same scheme as described in Ref. [4]. In the model under consideration here, the mass $m$ of each particle is taken to be the same, setting the time unit of the simulation $\tau_0 = \sqrt{\beta m \sigma_A^2}$. Similarly, the moments of inertia tensors of all particles were also chosen to be the same: $I_{xx} = I_{yy} = I_{zz} = m\sigma_A^2$.

During the equilibration of the simulations, the temperature is controlled by an Andersen thermostat: periodically, randomly selected particles are given a new velocity and angular velocity, drawn from a Maxwell-Boltzmann distribution. While measuring the diffusion coefficient, no thermostat is used, so that the total energy in the system is constant. To speed up equilibration of the system at low temperature, the initial configuration is taken from a standard canonical Monte Carlo simulation equilibrated at the same temperature $T$.

## WERTHEIM THEORY

Wertheim's thermodynamic perturbation theory allows us to obtain an analytical expression for the free energy of pure fluids and fluid mixtures (a detailed description can be found in Refs. [5, 6]). In the context of Wertheim's theory, and specialized to our system, the probability $p_\alpha$ that an $\alpha$-site ($\alpha \in \{A, B\}$) is bonded is obtained through the law of mass action, which in our case takes the form of a set of two coupled equations [7]:

$$p_A = 1 - \Big[1 + \rho\sigma_A^3 [4x_A(1-p_A)\Delta_{AA} + (1-x_A)(1-p_B)\Delta_{AB}]\Big]^{-1} \tag{5}$$

$$p_B = 1 - \left[1 + \rho\sigma_A^3[4x_A(1-p_A)\Delta_{AB}]\right]^{-1}, \qquad (6)$$

where $x_A = 0.2$ is the molar fraction of the species $A$, $\rho$ is the total number density. All interaction parameters needed for describing bonding between $AA$-and $AB$ enter in $\Delta_{AA}$ and $\Delta_{AB}$ :

$$\Delta_{AA} = g(\sigma_A)[\exp(\epsilon_{AA}/k_BT) - 1]\mathcal{V}_{AA}/\sigma_A^3 \qquad (7)$$

$$\Delta_{AB} = g(\sigma_{AB})[\exp(\epsilon_{AB}/k_BT) - 1]\mathcal{V}_{AB}/\sigma_A^3, \qquad (8)$$

where $\epsilon_{AA}$ and $\epsilon_{AB}$ are the bonding interaction energies of the $AA$-and $AB$-bonds. In the present work we have approximated $\Delta_{AA}$ and $\Delta_{AB}$ by using the contact values of the partial radial distribution functions [7], $g_{AA}(\sigma_A)$, $g_{BB}(\sigma_B)$, and $g_{AB}(\sigma_{AB})$ (where $\sigma_{AB} = (\sigma_A + \sigma_B)/2$), for a binary mixture of hard spheres as obtained from the Percus-Yevick Equation [8]:

$$g_{\alpha\alpha}(\sigma_\alpha) = \{(1-\xi) + \frac{3}{2}\sigma_\alpha X\}(1-\xi)^{-2} \;\; , \alpha \in \{A, B\} \qquad (9)$$

$$g_{AB}(\sigma_{AB}) = \left[\sigma_B g_{AA}(\sigma_A) + \sigma_A g_{BB}(\sigma_B)\right]/2\sigma_{AB}, \qquad (10)$$

where $\xi = \frac{\pi}{6}(\rho_A\sigma_A^3 + \rho_B\sigma_B^3)$, $X = \frac{\pi}{6}(\rho_A\sigma_A^2 + \rho_B\sigma_B^2)$, being $\rho_A$ and $\rho_B$ the partial number densities of the different species. The bonding volumes $\mathcal{V}_{AA}$ and $\mathcal{V}_{AB}$ present in Equations (7) and (8) are given by:

$$\mathcal{V}_{AA} = \frac{4\pi}{3}\left(\frac{1-\cos\theta_{AA}}{2}\right)^2\left[(\sigma_A + \delta_{AA})^3 - \sigma_A^3\right] \qquad (11)$$

$$\mathcal{V}_{AB} = \frac{4\pi}{3}\left(\frac{1-\cos\theta_{AB}}{2}\right)^2 \times$$
$$\times\left[(\sigma_{AB} + \delta_{AB})^3 - \sigma_{AB}^3\right], \qquad (12)$$

where $\delta_\gamma$ and $\theta_\gamma$ ($\gamma \in \{AA, AB\}$) are respectively the interaction ranges and the angular patch widths defined in the model section. Once Eqs. (5) and (6) are solved (by using Eqs. (7)-(12)), the probabilities $p_{\rm AA}$ and $p_{\rm AB}$ that an $A$-site is specifically bonded to another $A$- or to a $B$-site are obtained by the relations: $p_{\rm AA} = p_A - p_B$ and $p_{\rm AB} = p_B$.

## BOND PERSISTENCE

In this section we report results on the time evolution of the bond persistence function $p_b(t)$, i.e. the probability that a bond which is present at time zero is also present at time $t$, from which we obtained the decay time $\tau_b$ discussed in the main text according to the criterion $p_b(\tau_b) = e^{-1}$. The bonding persistence function $p_b(t)$ is defined as the number of bonds of the initial configuration for a given type $\alpha$ ($\alpha \in \{AA, AB\}$) which are still present at time $t$ normalized by the number of bonds of the same type $\alpha$ in the initial configuration.

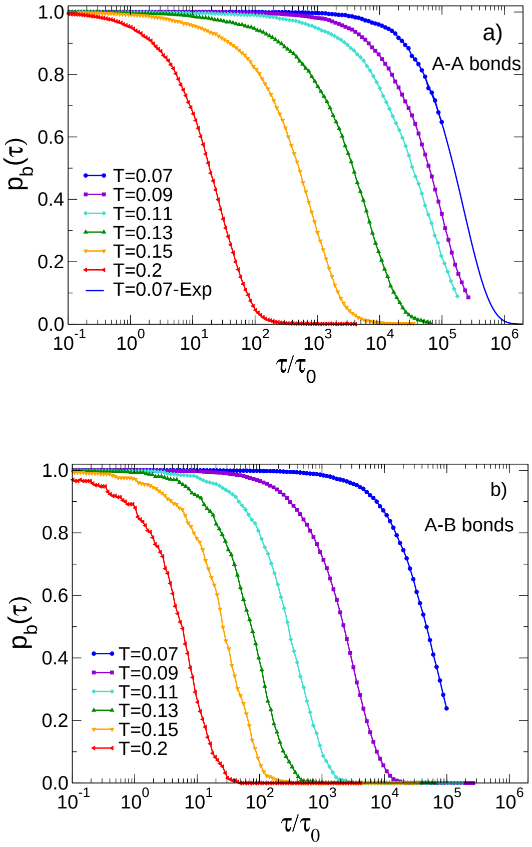


FIG. 1: a) Bond persistence function $p_b(\tau)$ of the $AA$-bond at different temperatures (different symbols) as a function of the dimensionless time $\tau/\tau_0$ where $\tau_0 = \sqrt{m_A\sigma_A^2/k_BT}$. We also include an example of extrapolation by means of an exponential function at $T = 0.07\epsilon_{AB}/k_B$ (blue solid line), b) Bond persistence function $p_b(\tau)$ of the $AB$-bond (symbols are as in a)).

Figures 1a and 1b show, respectively, $p_b(t)$ for $AA$- and $AB$-bonds at different temperatures. Due to the long computational time required, the values of $\tau_b$ at $T \leq 0.075\epsilon_{AB}/k_B$ for the $AA$-bond persistence and $T \leq 0.065\epsilon_{AB}/k_B$ for the $AB$-bond were obtained by extrapolation using an exponential function.


[1] N. Kern and D. Frenkel, J. Chem. Phys. **118**, 9882 (2003).
[2] D. C. Rapaport, Progress of Theoretical Physics Supplement **178**, 5 (2009).
[3] L. H. de la Peña, R. van Zon, J. Schofield, and S. B. Opps,

J. Chem. Phys **126**, 074105 (2007).
[4] F. Smallenburg and F. Sciortino, submitted (2013).
[5] M. S. Wertheim, J. Stat. Phys. **35**, 19 (1984).
[6] M. S. Wertheim, J. Stat. Phys. **35**, 35 (1984).
[7] D. de las Heras, J. M. Tavares, and M. M. Telo da Gama, Soft Matter **8**, 1785 (2012).
[8] J. L. Lebowitz and J. S. Rowlinson, J. Chem. Phys. **41**, 133 (1964).
